# Supplementary material for: Tunable nano-plasmonic photodetectors
Source: arXiv:2204.13978 source file (2022-04-29)
Supplement: Supplementary file 1 [file pertsch2022-tunable-preprint-SI.pdf]

# Tunable nano-plasmonic photodetectors - Supporting Information

Patrick Pertsch, René Kullock, Vinzenz Gabriel, Luka Zurak, Monika Emmerling,  
and Bert Hecht\*

*NanoOptics & Biophotonics Group, Experimental Physics 5, University of Würzburg, Am  
Hubland, 97074 Würzburg, Germany*

E-mail: hecht@physik.uni-wuerzburg.de

## Sample Fabrication

The antennas are structured from mono-crystalline gold platelets that are grown in a wet-chemical process on glass.<sup>1</sup> In a first step, they are transferred to another glass substrate with evaporated gold contacts. Details on the transfer can be found elsewhere.<sup>2</sup> The platelets are then structured by focused ion beam milling in a Zeiss "ORION NanoFab" system with He- and Ga-ions. Ga-ions were used for coarse milling, while He-ions were used for the fine structuring of the antennas. An exemplary sample is shown in figure S1.

The prepared antennas were immediately coated with the thin  $\text{AlO}_x$  passivation layer and the  $\text{TiO}_x$  by atomic layer deposition (Anric Technologies AT-410).  $\text{AlO}_x$  films are prepared from TMA (Trimethylaluminium, Sigma-Aldrich) and  $\text{H}_2\text{O}$  precursors at  $90^\circ$  (5 cycles),  $\text{TiO}_x$  with TDMAT (Tetrakis-(dimethylamido)-titan, Sigma-Aldrich) and  $\text{H}_2\text{O}$  at  $100^\circ$  (400 cycles).

The usual growth rate for  $\text{AlO}_x$  is about 0.1 nm per cycle resulting in a passivation layer of  $\sim 0.5$  nm. The thickness of the  $\text{TiO}_x$  films was determined from SEM images and varies between 25-30 nm.

To allow electrical contact to the sample, a mask was used during the ALD process, shielding the contact pads against the coating.

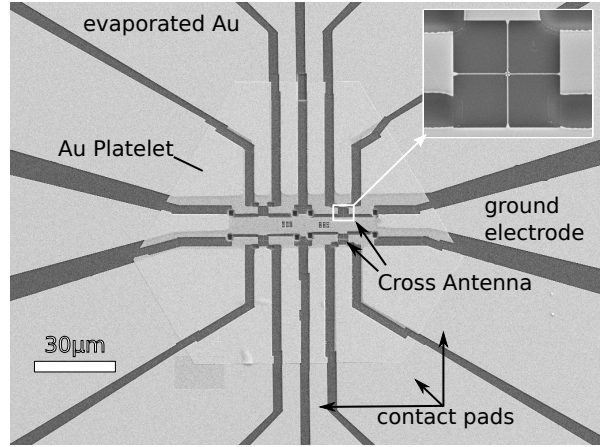

Fig. S 1: Structured gold platelet with four cross antennas on evaporated gold electrodes. The inset shows one of the antennas with connection wires. Each antenna in this image is connected to three contact pads and the ground electrode. Dimer antennas are only connected via one contact pad and the ground electrode (not shown).

## Dark Current

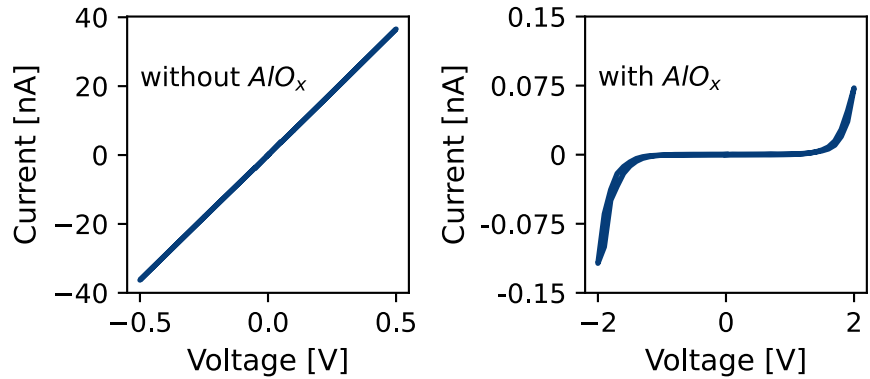

Fig. S 2: Comparison of the dark currents of an antenna without  $\text{AlO}_x$  (left) and with  $\text{AlO}_x$  passivation layer (right).

In a first series of experiments, the antennas were coated directly with  $\text{TiO}_x$ , without any passivation layer. However this resulted in the ohmic contact behavior observed in figure S2.

By heating the sample to 250°C for 48 h, this dark current was reduced significantly (not shown). But because the antennas tend to deform at these high temperatures, we decided to use an  $\text{AlO}_x$  passivation layer similar to García de Arquer et al.,<sup>3</sup> which drastically reduces the dark current without additional heating of the sample.

The dark current measurements were recorded with a Keithley 2604B source-meter (Tektronix Inc.).

## Schottky-Barrier

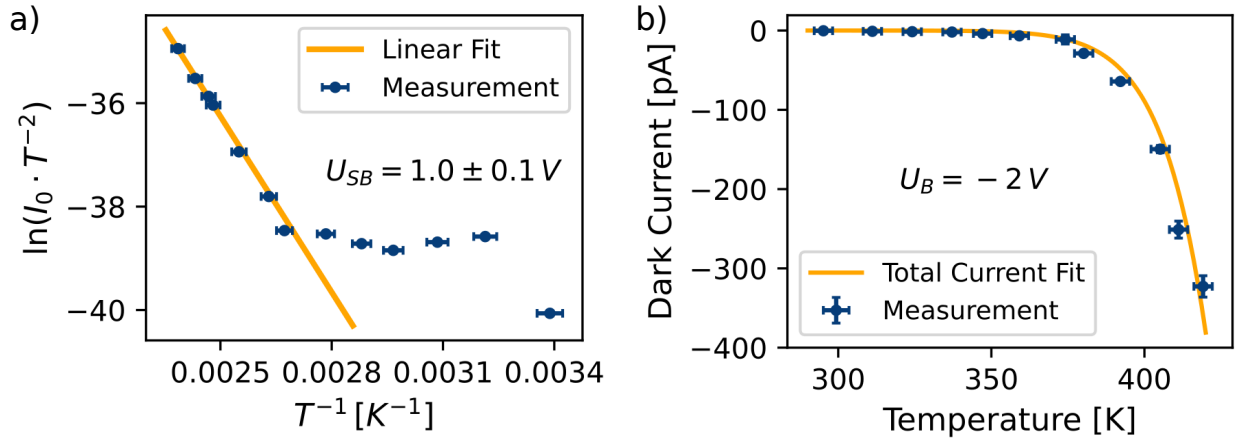

Fig. S 3: Temperature dependent dark current experiments. a) Linearized saturation current  $I_0$  over inverse temperature  $T^{-1}$ . A linear curve is fitted to the data to obtain the Schottky-barrier height  $U_{SB}$  from the slope. b) shows the dark current at a bias voltage of  $U_B = -2 \text{ V}$  as a function of the temperature. The total current according to equation 1 is fitted to the data.

To estimate the Schottky-barrier height in the metal-semiconductor-metal (MSM) devices we follow the approach proposed by Averine et al.<sup>4</sup> The dark current  $I_D$  is measured as a function of the applied bias voltage  $U_B$  at different temperatures  $T$ . In this configuration, always one of the two Schottky-barriers of the MSM-structure is in reverse bias, therefore the current is limited by the thermionic emission over the barrier. The increase in current with increased bias is a result of the lowered Schottky-barrier by the electric field. This is

described by

$$I_D = I_0 \exp\left(\frac{eU_B}{nk_B T}\right) [1 - \exp\left(\frac{-eU_B}{k_B T}\right)] \quad (1)$$

with

$$I_0 = A^* S T^2 \exp\left(\frac{-eU_{SB}}{k_B T}\right), \quad (2)$$

where  $U_{SB}$  is the height of the Schottky-barrier, and  $n$  is the ideality factor, and  $k_B$  and  $e$  are the Boltzmann-constant and the elementary charge, respectively. The saturation current  $I_0$  is proportional to the effective Richardson-constant  $A^*$ , and the surface of the contact  $S$ .  $I_0$  and  $n$  are obtained from  $I_D(U_B)$  measurements at different temperatures. Since the saturation current depends on the  $U_{SB}$  and  $T$ , we can obtain  $U_{SB}$  by plotting  $\ln(I_0 \cdot T^{-2})$  over  $T^{-1}$  and fitting a linear curve to the data (Fig. S3 a). We only fit the temperature range above 370 K, since the measured dark currents at lower temperatures are close to the detection limit of our measurement device and, hence, the data points are less reliable at low temperatures. From the high temperature data points we derive the Schottky-barrier height

$$U_{SB} = (1.0 \pm 0.1) \text{ eV}.$$

With the obtained values for  $U_{SB}$  and  $n$  we fit the data in figure S3 b, using equation 1 and with only one free parameter  $a = A^* S$ , showing good agreement between measurement and theory.

## Photocurrent measurements

**Photocurrent spectrum** The photocurrent spectra were recorded by exciting the antennas with monochromatic light and sweeping the wavelength from 900 nm to 500 nm (or vice versa) in steps of 5 nm. A supercontinuum laser (NKT Photonics, SuperK FIANIUM FIU-15) was used as light source with an acousto-optic tunable filter (AOTF) to select specific wavelengths (NKT Photonics, SuperK SELECT). The AOTF transmission was calibrated

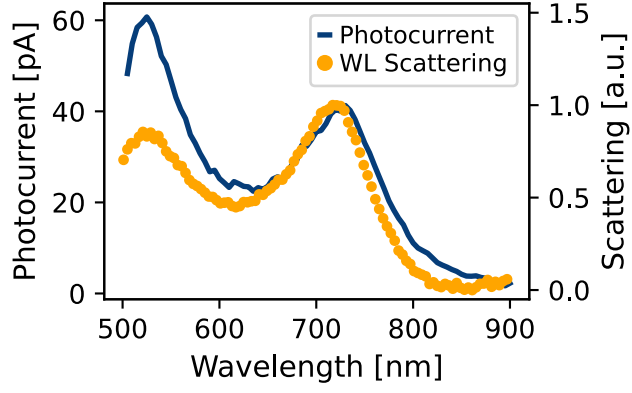

Fig. S 4: Full photocurrent spectrum of a symmetric dimer antenna (blue) with the corresponding white light (WL) scattering spectrum (orange). In addition to the antenna resonance at 700 nm, also the connector features a resonance at wavelengths below 600 nm.

to achieve constant light power on the sample over the whole wavelength range. If not mentioned otherwise, the laser polarization was chosen to be parallel to the antenna axis.

The laser beam is passed through a 300  $\mu\text{m}$  pinhole that is imaged on the backfocal-plane of the objective (Nikon 100x, NA 1.45) resulting in a collimated spot at the sample with a diameter of  $\sim 1.5 \mu\text{m}$ .

The photocurrent at each wavelength is recorded with a Keithley 2636B source meter (Tektronix Inc.), which is also used to apply the bias voltage to the sample. Before the sweep is started, the bias voltage is already applied while the dark current is measured for a specific time (usually 30s), to allow charging/discharging of any capacitance in the system. This dark current is subtracted from the obtained photocurrent.

The spectra shown in the main text represent the mean value of 3-5 single spectra to reduce noise in the measurement.

**Polarization pattern** To measure the photocurrent  $I_{Ph}$  as a function of the laser polarization, an achromatic half-wave plate and a linear polarization filter are introduced to the beam path (behind the pinhole). The polarization filter defines the angle  $\Phi$  of the laser polarization while the half-wave plate is used to regulate the laser power to a specific level (measured directly after the polarization filter). To obtain the polarization patterns, the

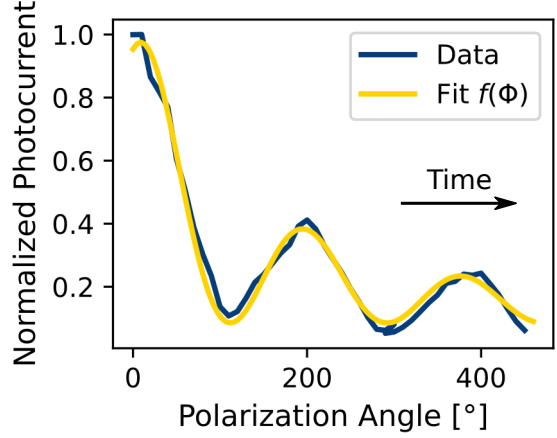

Fig. S 5: Time correction of the polarization pattern for the symmetric antenna. The duration of the complete measurement (starting at 0° and ending at 450°) was about 75 minutes. The times between different angles were comparable.

filter is rotated while keeping the laser power and the wavelength constant.

Since the photocurrent of our antennas slowly decreases over time  $t$ , a correction is necessary to obtain the polarization pattern. To this end, we split  $I_{Ph}(\Phi, t) = T(t) \cdot I_{Ph}(\Phi) = f(\Phi(t))$  into a (bi-exponential) time decay  $T(t) = T(\Phi(t))$  and the sought after angular dependence  $I_{Ph}(\Phi)$ . For the latter we assume the previously reported  $\cos(\Phi)^2$  pattern,<sup>5</sup> which fits well to our data. The data is then corrected by fitting  $f(\Phi) = (\exp(-\beta_1\Phi) + \exp(-\beta_2\Phi)) \cdot \cos(\Phi - \Phi_0)^2$  to the measurement values, and dividing the original values by the obtained bi-exponential decay.

This is only done for the dimer antennas, since a correction is not necessary for the cross- and trimer-antennas, due to the normalization to the total current.

## Numerical Simulations

The FEM simulations discussed in the main text were performed by using COMSOL Multiphysics<sup>®</sup>.<sup>6</sup> We used the “Wave Optics Module” to solve Maxwell’s equations in frequency domain for the field scattered by a gold nanoantenna. For all scenarios under consideration, the structure is placed on top of a glass substrate. Structure and substrate are covered

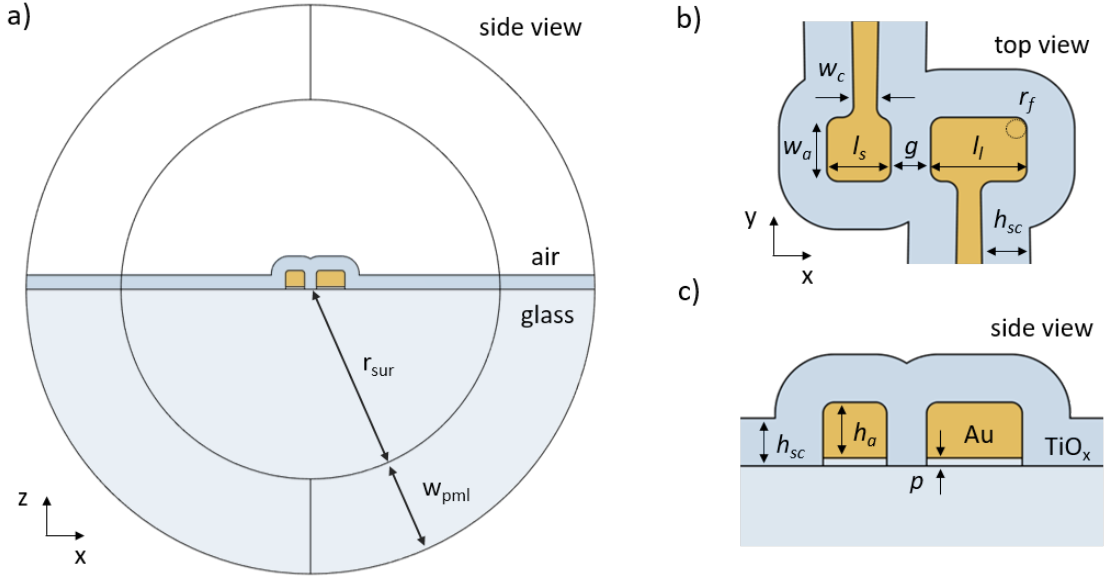

Fig. S 6: Geometry outline of the COMSOL simulations. a) Side view of the complete geometry. b) Top view of the antenna area. Denoted quantities are:  $w_c$  – connector width,  $w_a$  – antenna width,  $l_s$  – length of the short rod,  $g$  – gap size,  $l_l$  – length of the long rod,  $r_f$  – radius of curvature,  $h_{sc}$  – height of the coating layer. c) Side view zoom-in. Denoted quantities are:  $h_a$  – height of the antenna,  $p$  – height of the glass pedestal.

with 35 nm of TiOx (S6 a). A plane wave propagating in  $+z$  direction is used as excitation field (background field). Due to presence of the interface, the background field in the upper hemisphere is calculated from Fresnel coefficients, neglecting the presence of the antenna and the coating layer. Refractive indices of glass and TiOx were kept constant in the simulated spectral interval ranging from 500 up to 1000 nm and were equal to 1.52 and 2 respectively. The permittivity of gold was modeled using experimental data from Olmon et al.,<sup>7</sup> as it has been demonstrated to accurately represent the optical response of our gold platelets.<sup>8</sup> The simulation region, as in the exemplary case shown in Fig. S6 a), is a sphere with radius of 600 nm, where the volume surrounding the antenna has a radius  $r_{sur} = 400$  nm. In addition, a perfectly matched layer (pml) with thickness  $w_{pml} = 200$  nm is introduced, an absorbing layer which is added to mimic an open and nonreflecting infinite domain. The dimensions of the antenna, which can be seen in the top view (S6 b), have been taken from SEM images (see main text, Fig. 3a). Some of the quantities could only be estimated with some

uncertainty (antenna thickness, height of the pedestal), leaving a range of values to match the experimentally observed spectra (S6 c).

## Cross Antenna

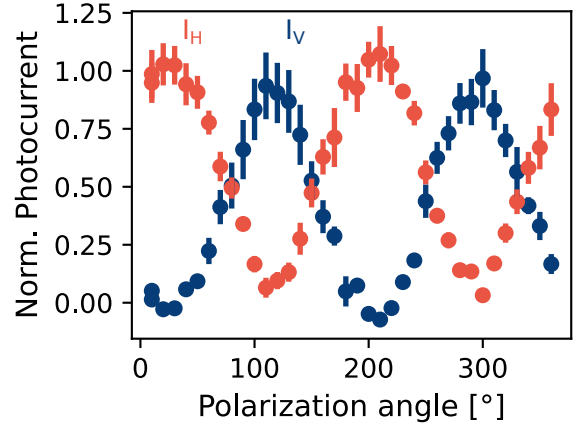

Fig. S 7: Polarization dependence of the cross antenna of Fig. 4 (main text). The currents are normalized to the total current ( $I_H + I_V$ ).

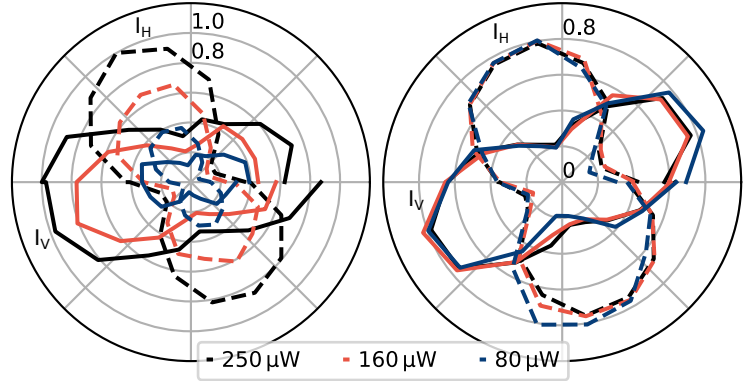

Fig. S 8: Polarization pattern of a cross antenna for three different laser powers ( $250 \mu W$ ,  $160 \mu W$  and  $80 \mu W$ ), normalized to the maximum photocurrent (left) or to ( $I_H + I_V$ ) (right).

To show that the cross antenna polarization patterns do not depend on the light intensity, we recorded the patterns for three different laser powers. Note that these measurements were

done on a different cross antenna, not shown in the main paper. The resonance of this antenna was at 750 nm, therefore the measurements were recorded at this wavelength. On the left side of Fig. S8 the photocurrent was normalized to the maximum current at the highest power of 250  $\mu$ W. From this plot it is obvious that the absolute current of the two dimers indeed depends on the incident light power, and that it decreases over time. However, the photocurrent normalized to the total current  $I_H + I_V$ , in the right plot of the figure, shows no significant difference between the three laser powers. Hence this result confirms that no intensity calibration is needed for our polarization detectors based on the cross antennas.

## Trimer Antenna

As mentioned in the main text, the polarization detection with the cross antennas is ambiguous, since a polarization rotation by 90° leads to the same photocurrent. We can overcome this problem by using an antenna with three fold symmetry, like the one displayed in Fig. S9. This "Trimer" antenna consists of three antenna arms (M1-M3) rotated by 120° with respect to each other. This way, only a polarization rotation by 180° leads to the same measured photocurrent. Therefore, by comparing the currents through M1-M3, the polarization can be determined unambiguously.

Due to experimental restrictions, only two currents could be measured at the same time. Also, to apply the bias voltage, a counter electrode was necessary. Because of this, M3 was grounded for all measurements. To still obtain the photocurrent of all three arms, the measurement is split up in time: For negative bias the hot electrons flow away from M1 and M2 and are collected by M3. Thus the photocurrent of M1 and M2 can be directly measured through the top connection wires for negative bias. For positive bias the hot electrons flow away from M3 and are collected by the other two arms. Hence, the current through M3 can be computed for positive bias by summing the currents through the top connection wires.

This approach yields the expected polarization dependence for the photocurrent of the

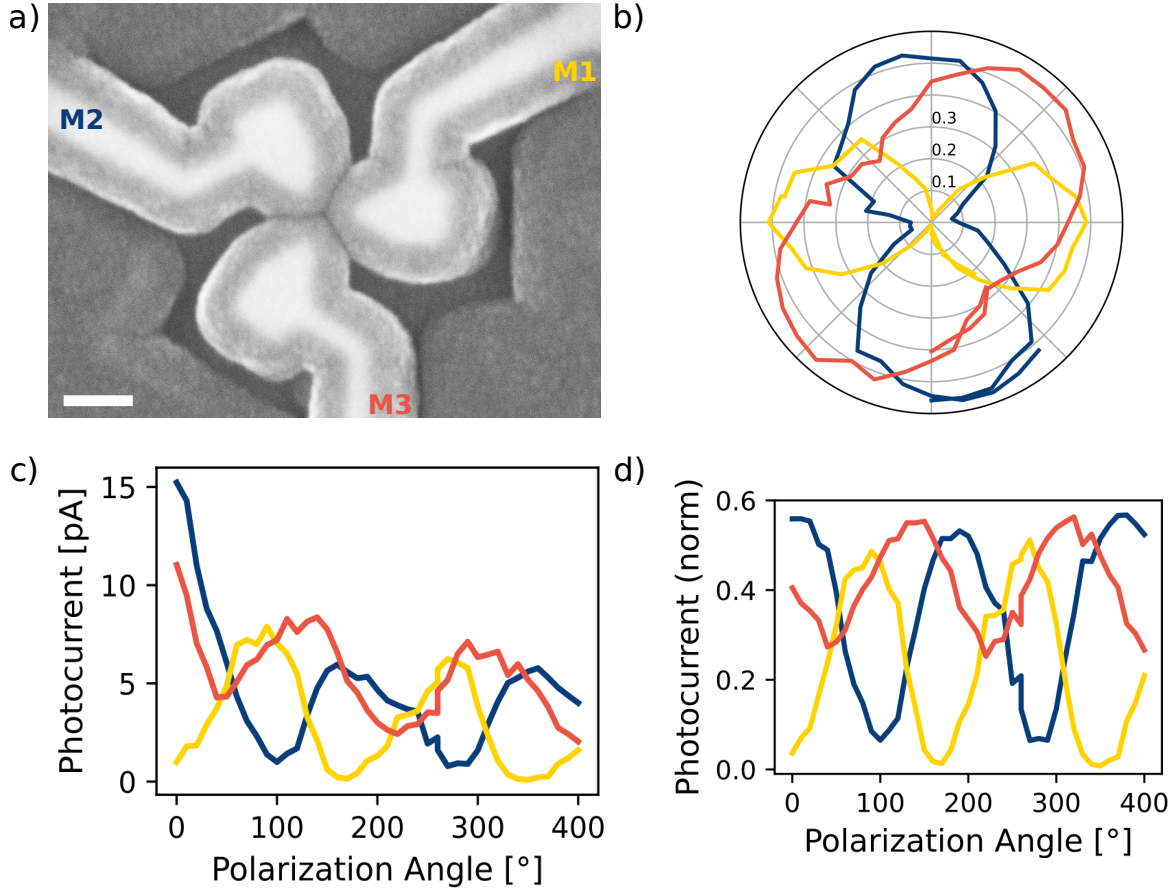

Fig. S 9: SEM image of a trimer antenna a). Polarization dependence of the photocurrent through M1-M3, in polar b) and cartesian coordinates c) and d). c) shows the absolute values from the measurement, while the graphs in b) and d) are normalized to the total current (M1+M2+M3).

three antenna arms. But its obvious from graph b) and d) that the minimum current in M3 is higher than for M1 and M2. This could be explained by an asymmetry in the photocurrent under switching of the polarity. In the future, more advanced measurement approaches are expected to result in more symmetric currents through the three antenna arms, e.g. by splitting the measurement into three parts and grounding always two of the connection wires instead of only one.

## Efficiency Calculation

To estimate the efficiency of our device we use the photocurrent of the symmetric dimer in figure S4,  $I_{Ph} \approx 40 \cdot 10^{-12}$  A, at the resonance wavelength  $\lambda \approx 725$  nm.

We compute the external quantum efficiency via

$$\eta_{ext} = \frac{n_{e^-}}{n_{Ph}} = \frac{I_{Ph}}{P_{tot}} \frac{hc}{\lambda e} \approx 10^{-6}$$

, where  $n_{e^-}$  and  $n_{Ph}$  are the number of electrons and photons per second,  $h$  is the Planck-constant and  $c$  the speed of light. The total laser power was  $P_{tot} = 40 \mu\text{W}$  during the measurement.

Due to the mismatch between the area of the laser spot  $A_L$  and antenna absorption cross section  $\sigma_A$ , most of the light cannot be absorbed by the antenna. To attribute for this, we correct the quantum efficiency by an absorption factor ( $A_L/\sigma_A$ ). With this factor the corrected quantum efficiency computes to

$$\eta = \eta_{ext} \cdot (A_L/\sigma_A) \approx 10^{-4}.$$

For this we used  $\sigma_A \approx 10^{-14} \text{ m}^2$ , which we obtained from our simulations, and computed the laser spot area from its diameter  $d \approx 1.5 \mu\text{m}$ .

## References

- (1) Krauss, E.; Kullock, R.; Wu, X.; Geisler, P.; Lundt, N.; Kamp, M.; Hecht, B. Controlled Growth of High-Aspect-Ratio Single-Crystalline Gold Platelets. *Crystal Growth & Design* **2018**, *18*, 1297–1302.
- (2) Kullock, R.; Ochs, M.; Grimm, P.; Emmerling, M.; Hecht, B. Electrically-driven Yagi-Uda antennas for light. *Nature Communications* **2020**, *11*, 1–7.

- (3) García de Arquer, F. P.; Mihi, A.; Kufer, D.; Konstantatos, G. Photoelectric Energy Conversion of Plasmon-Generated Hot Carriers in Metal–Insulator–Semiconductor Structures. *ACS Nano* **2013**, *7*, 3581–3588.
- (4) Averine, S.; Chan, Y. C.; Lam, Y. L. Evaluation of Schottky contact parameters in metal–semiconductor–metal photodiode structures. *Applied Physics Letters* **2000**, *77*, 274–276.
- (5) Knight, M. W.; Sobhani, H.; Nordlander, P.; Halas, N. J. Photodetection with Active Optical Antennas. *Science* **2011**, *332*, 702–704.
- (6) COMSOL Multiphysics® v. 5.6. [www.comsol.com](http://www.comsol.com), Stockholm, Sweden.
- (7) Olmon, R. L.; Slovick, B.; Johnson, T. W.; Shelton, D.; Oh, S.-H.; Boreman, G. D.; Raschke, M. B. Optical dielectric function of gold. *Physical Review B* **2012**, *86*, 235147.
- (8) Großmann, S.; Friedrich, D.; Karolak, M.; Kullock, R.; Krauss, E.; Emmerling, M.; Sangiovanni, G.; Hecht, B. Nonclassical Optical Properties of Mesoscopic Gold. *Physical Review Letters* **2019**, *122*, 246802.
